# Supplementary material for: VersiCode: Towards Version-controllable Code Generation
Source: arXiv:2406.07411 source file (2024-10-16)
Supplement: Supplementary file 4 [file D_evaluation_details.tex]

\section{Evaluation Details}
\label{apd:evaluation_details}
\subsection{Hyper-parameter}
\label{subapd:parameter}

As illustrated in Table~\ref{tab:hyper}, we have itemized the hyper-parameters pertinent to version-controllable code generation.

\begin{table}[t]
\centering
\caption{Hyper-parameters for completion and editing.\label{tab:hyper}}
\resizebox{.5\textwidth}{!}{
\begin{tabular}{@{}ccccc@{}}
\toprule
\multirow{2}{*}{\textbf{hyper-parameter}} & \multicolumn{3}{c}{\textbf{code completion}} & \textbf{code editing} \\
\cmidrule(l){2-4}\cmidrule(l){5-5}
                                 & token-level   & line-level   & block-level   & block-level           \\
                            \midrule
temperature                      & 0.8           & 0.8          & 0.8           & 0.8                   \\
top\_p                           & 0.95          & 0.95         & 0.95          & 0.95                  \\
max\_tokens                      & 64            & 128          & 512           & 512                   \\
n                                & 100           & 6            & 6             & 6     \\      
\bottomrule
\end{tabular}}
\end{table}



\subsection{Prompt Template}
\label{subapd:prompt}


We introduce the prompt template for token-level, line-level, and block-level evaluations in Figure~\ref{fig:token_prompt}, Figure~\ref{fig:line-template}, and Figure~\ref{fig:block-template}, respectively.


\begin{figure}[t]
    \centering
    \includegraphics[width=1.0\textwidth, bb=0 0 741 296.67]{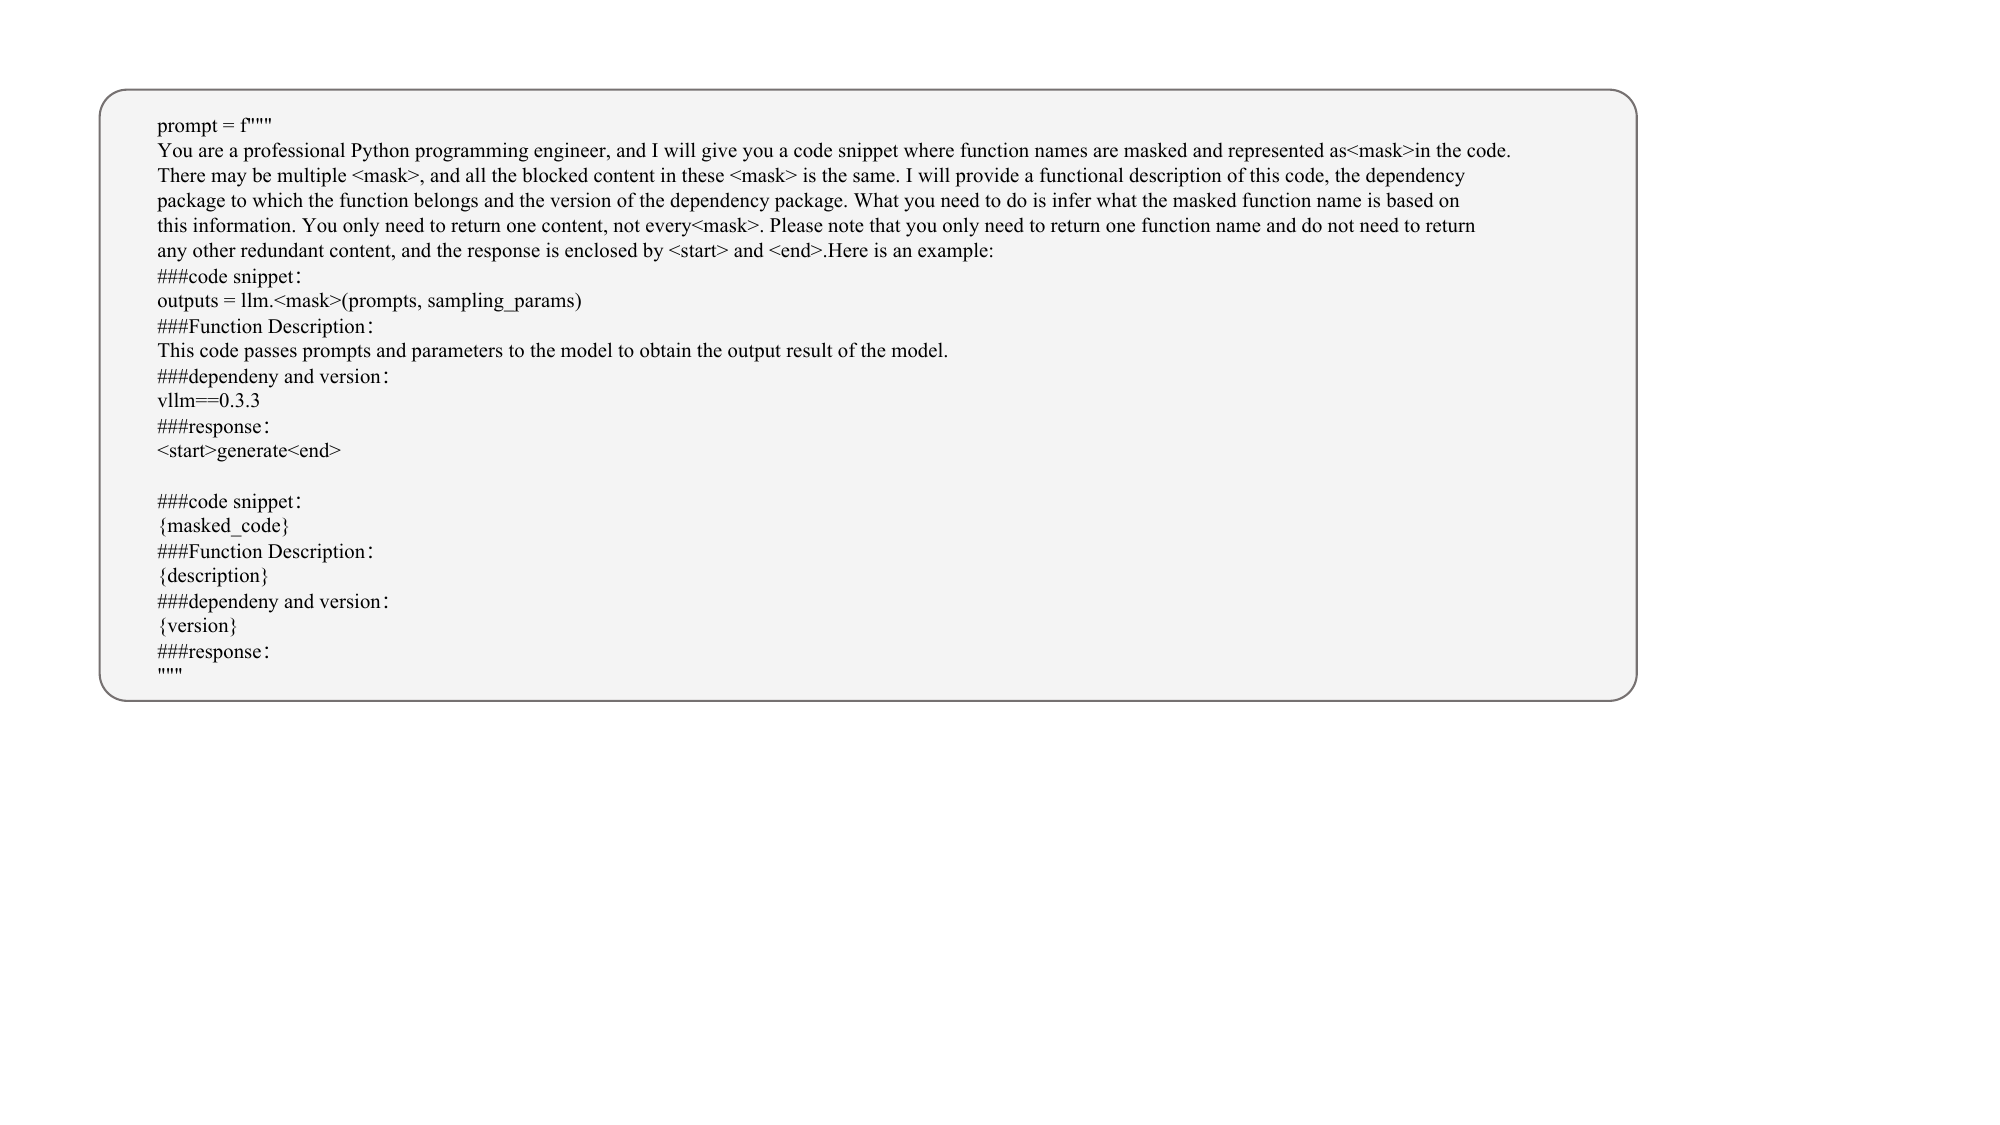}
    \caption{Prompt template for token-level version-specific code completion.}
    \label{fig:token_prompt}
\end{figure}

\begin{figure}[t]
    \centering
    \includegraphics[width=1.0\textwidth, bb=0 0 741.43 332.70]{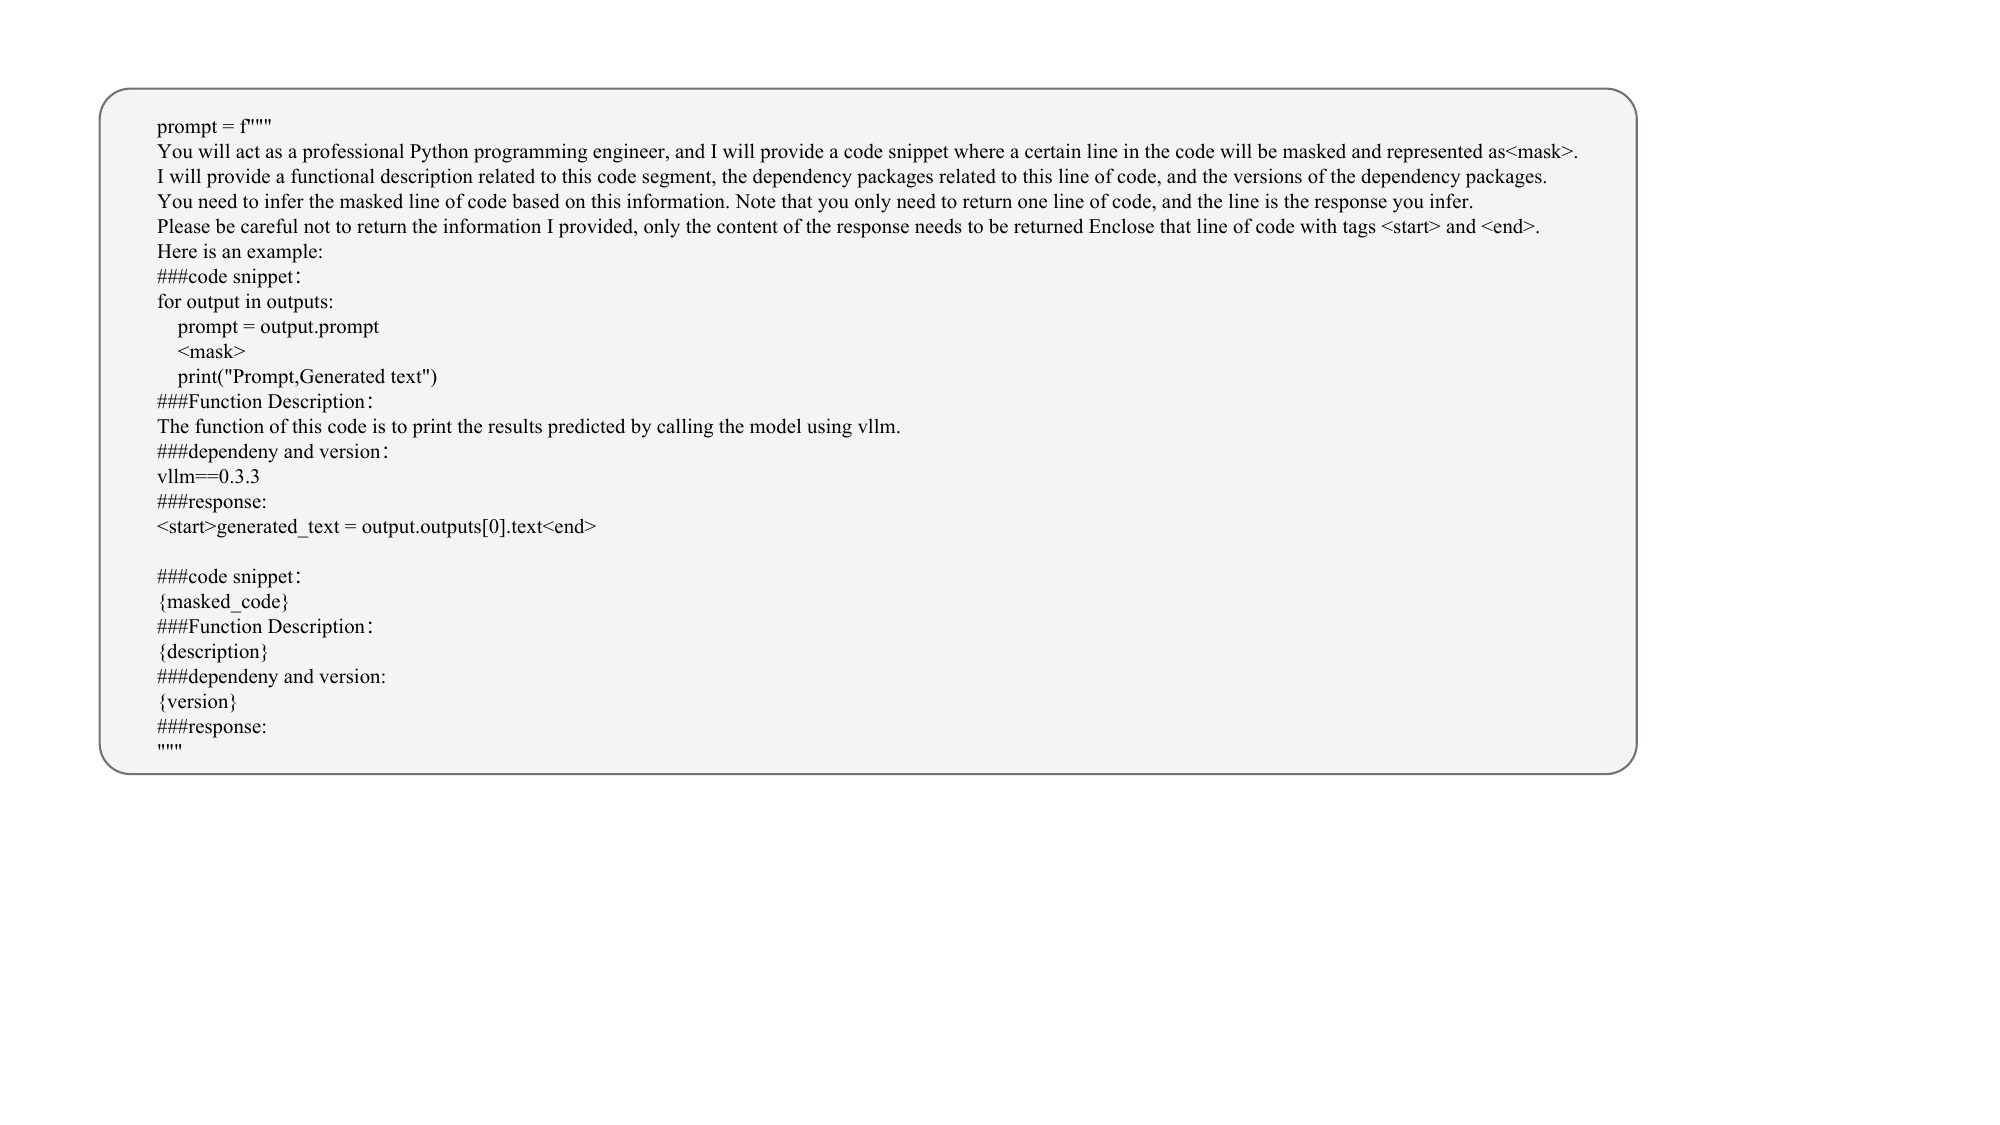}
    \caption{Prompt template for line-level version-specific code completion.}
    \label{fig:line-template}
\end{figure}


\begin{figure}[t]
    \centering
    \includegraphics[width=1.0\textwidth, bb=0 0 741 300.87]{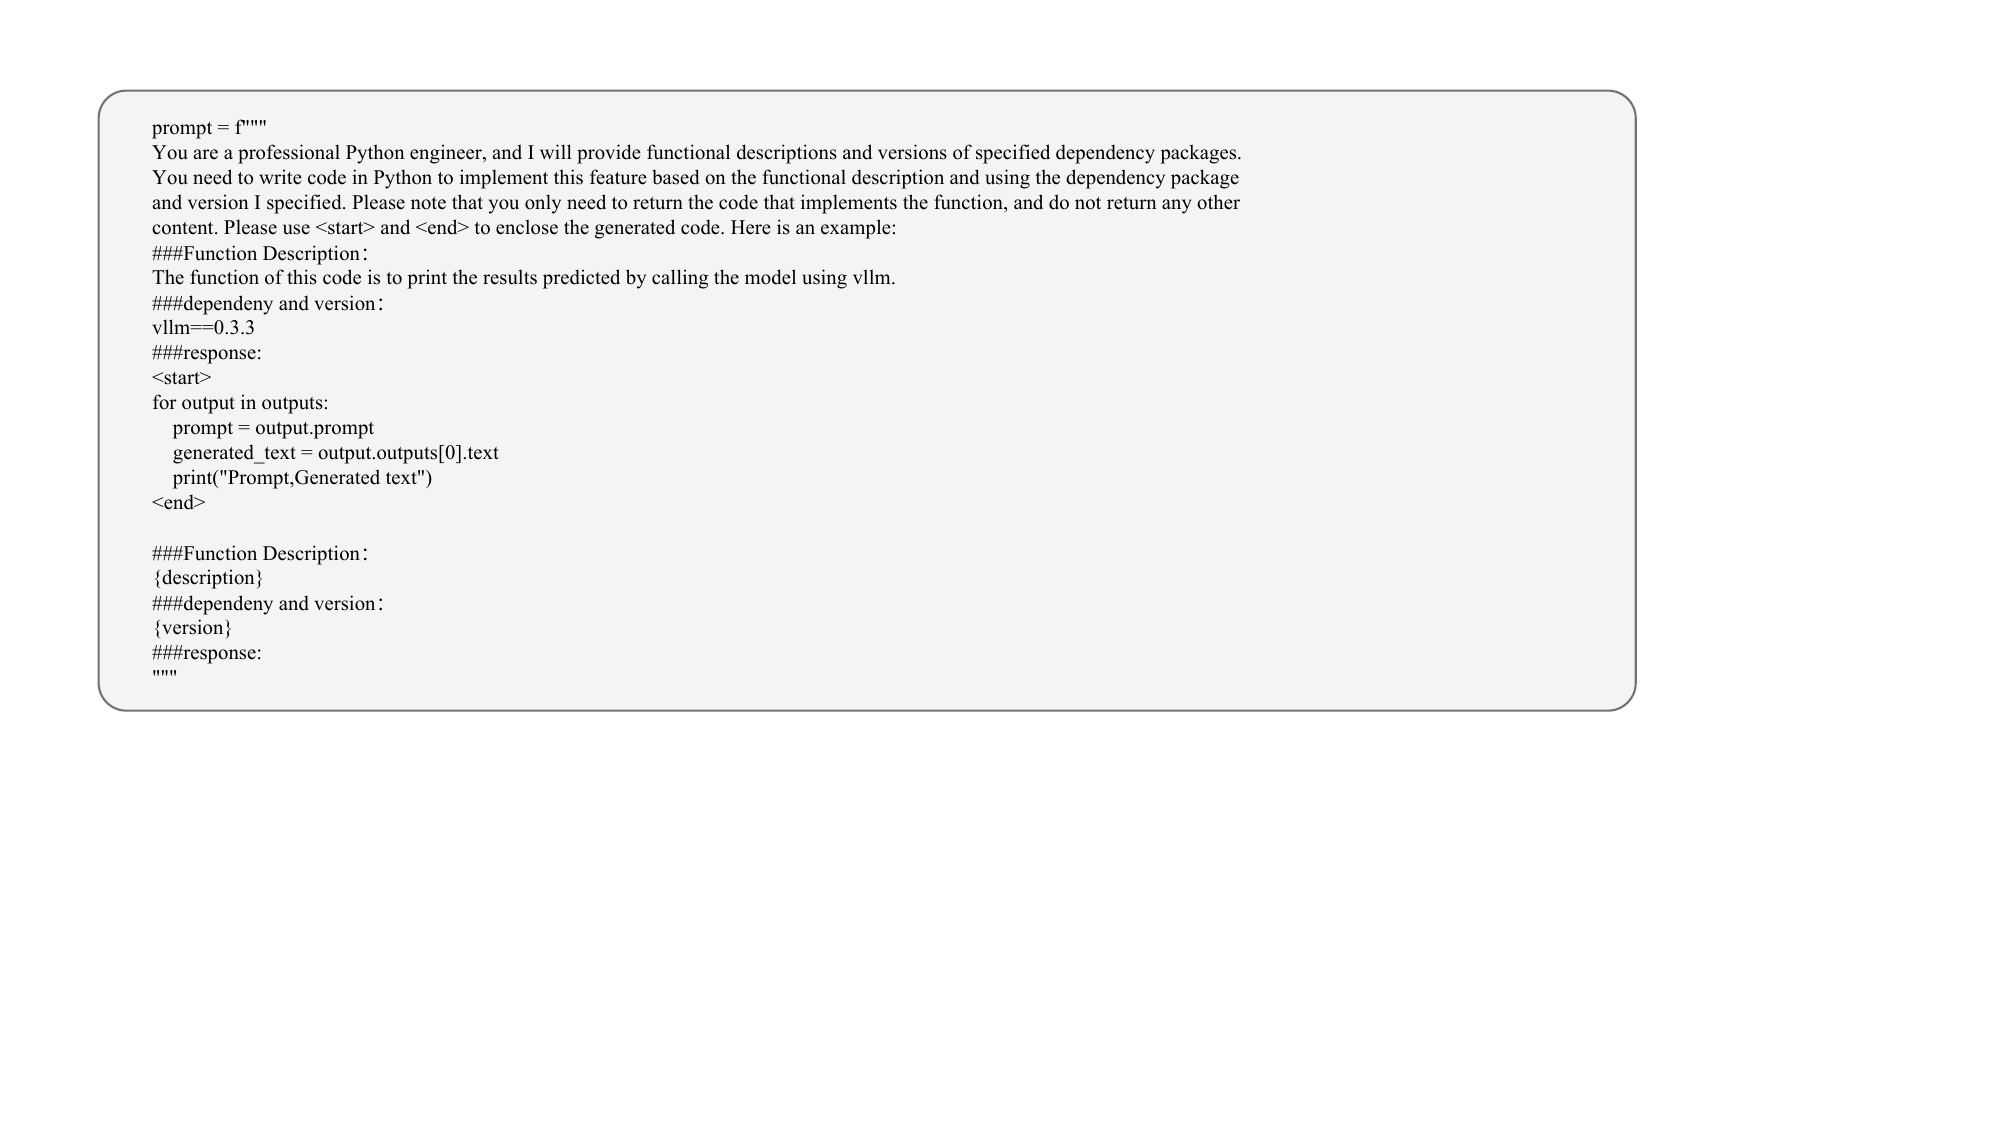}
    \caption{Prompt template for block-level version-specific code completion.}
    \label{fig:block-template}
\end{figure}

\begin{figure}
    \centering
    \includegraphics[width=1.0\textwidth, bb=0 0 741.43 205.38]{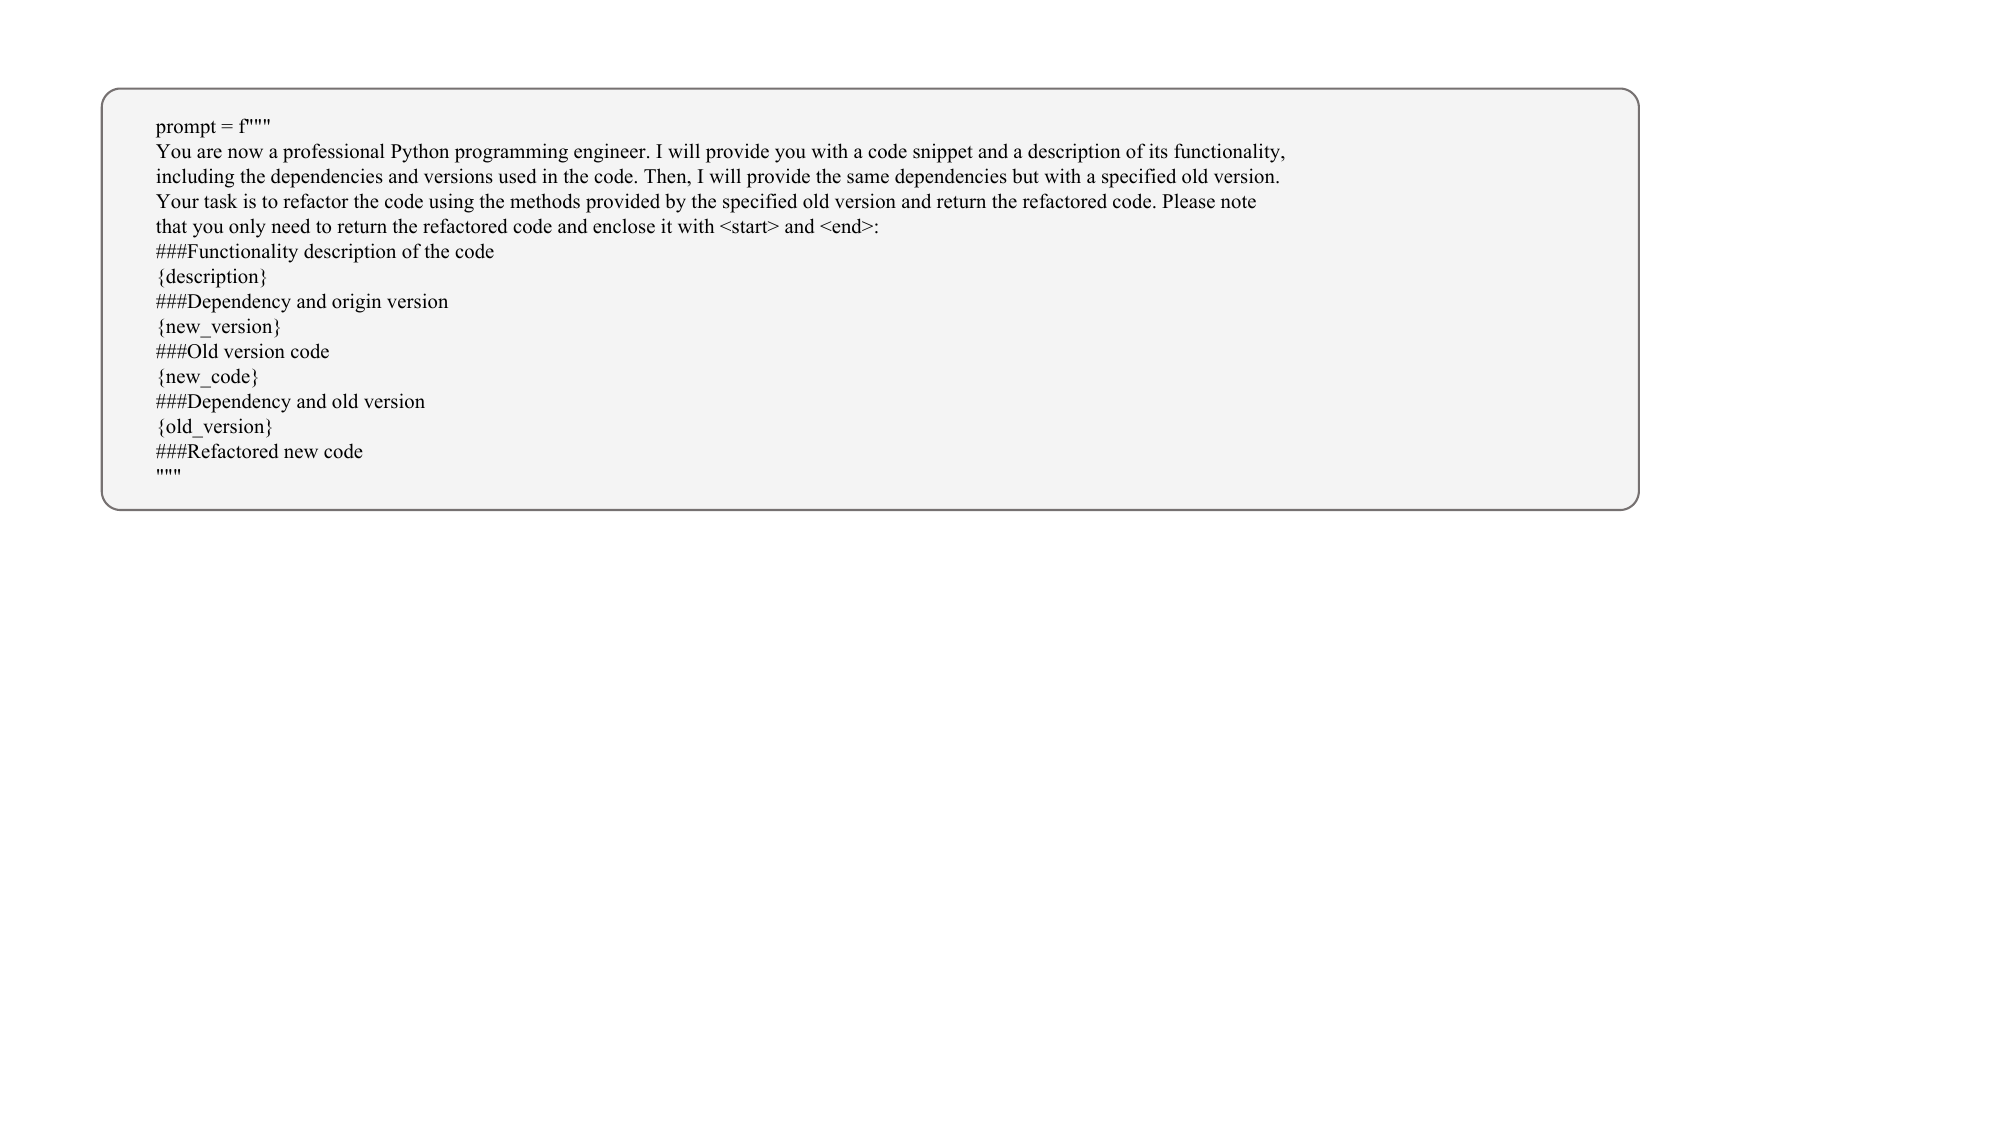}
    \caption{Prompt template for version-aware code editing.}
    \label{fig:enter-label}
\end{figure}


\subsection{Data Sampling}
\label{subapd:sample}
For token and line-level tasks, we randomly sampled 2,000 instances for evaluation. For block-level tasks, we used the entire dataset due to its smaller size. In the time trend experiment, we sampled 200 data points per quarter or used all available data if fewer.
