# Supplementary material for: VersiCode: Towards Version-controllable Code Generation
Source: arXiv:2406.07411 source file (2024-10-16)
Supplement: Supplementary file 5 [file E_examples.tex]

\section{Executable Test Case}
\label{apd:executable_test_case}
\tong{add description of task description and associated test cases.}

\begin{figure*}
    \centering
    \includegraphics[width=\linewidth]{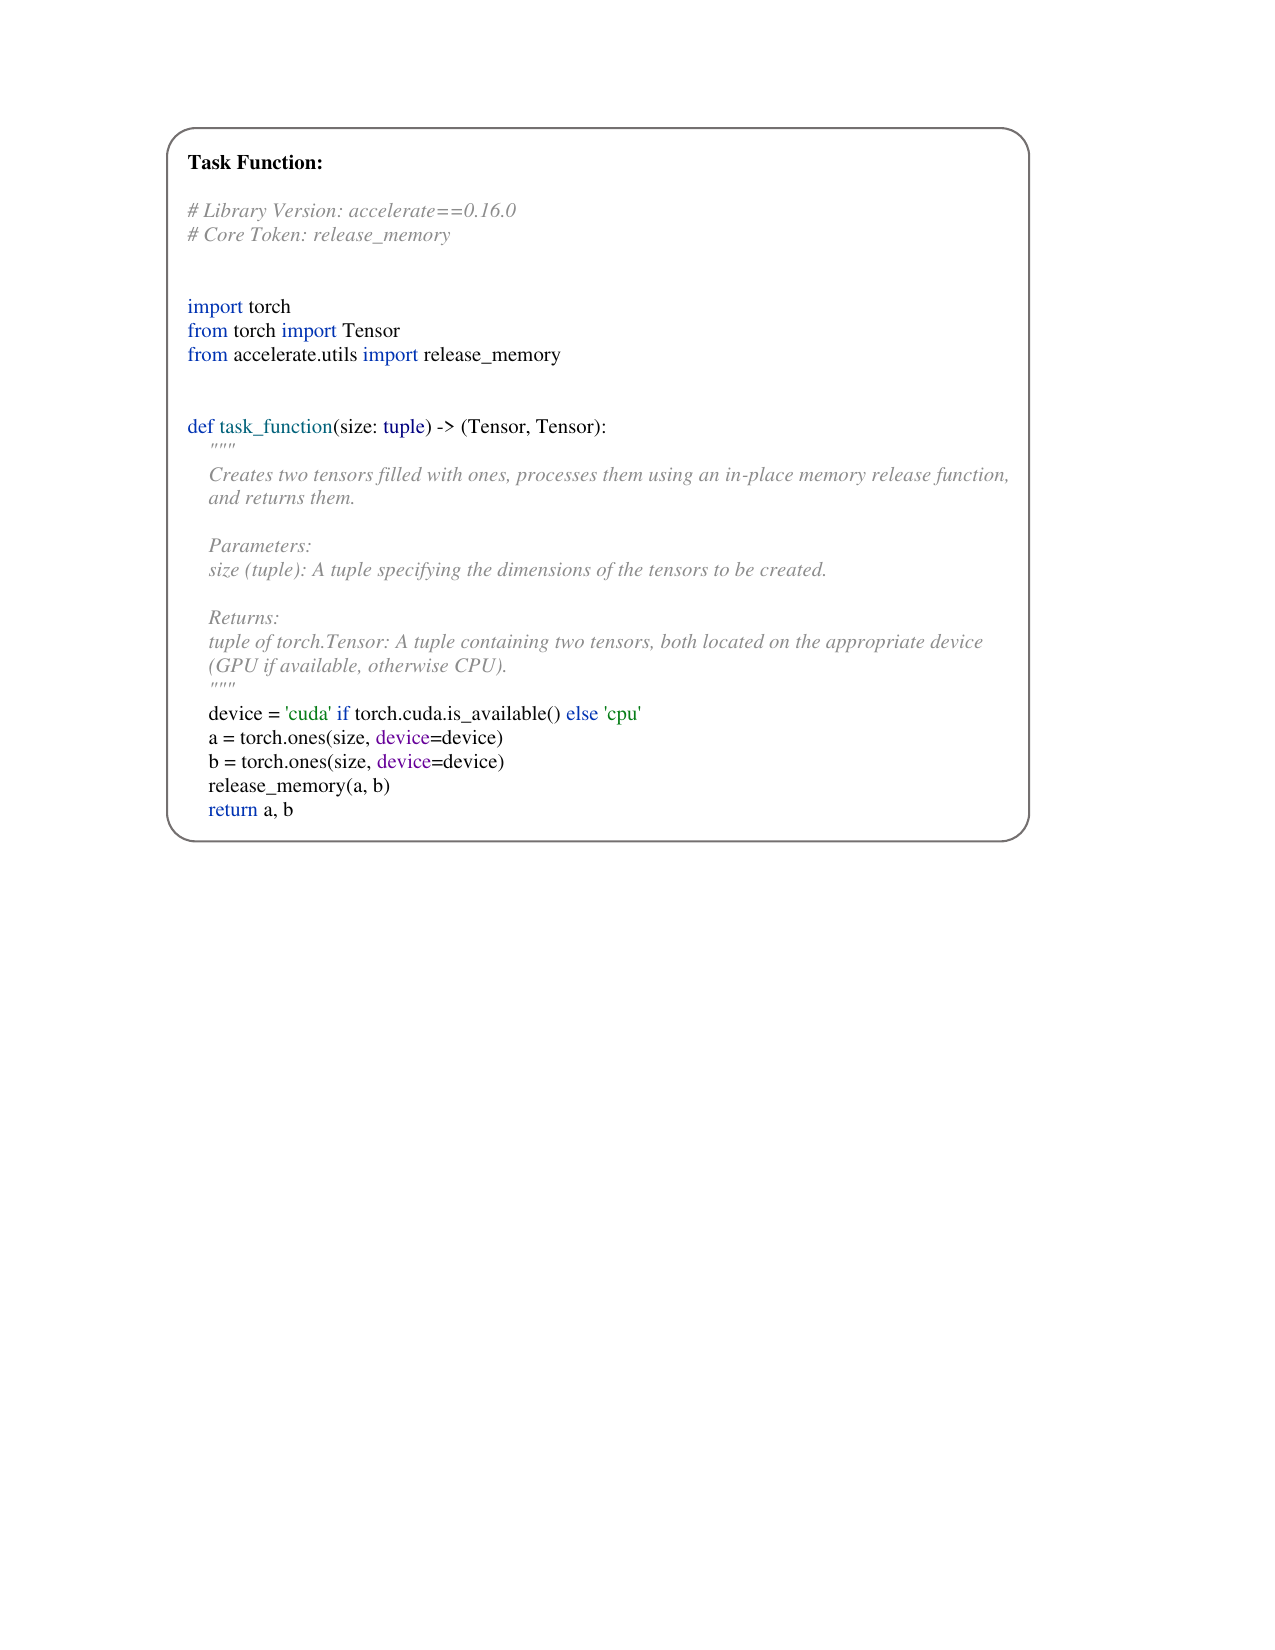}
    \caption{An example of function signature.}
    \label{fig:task_signature}
\end{figure*}


\begin{figure*}
    \centering
    \includegraphics[width=\linewidth]{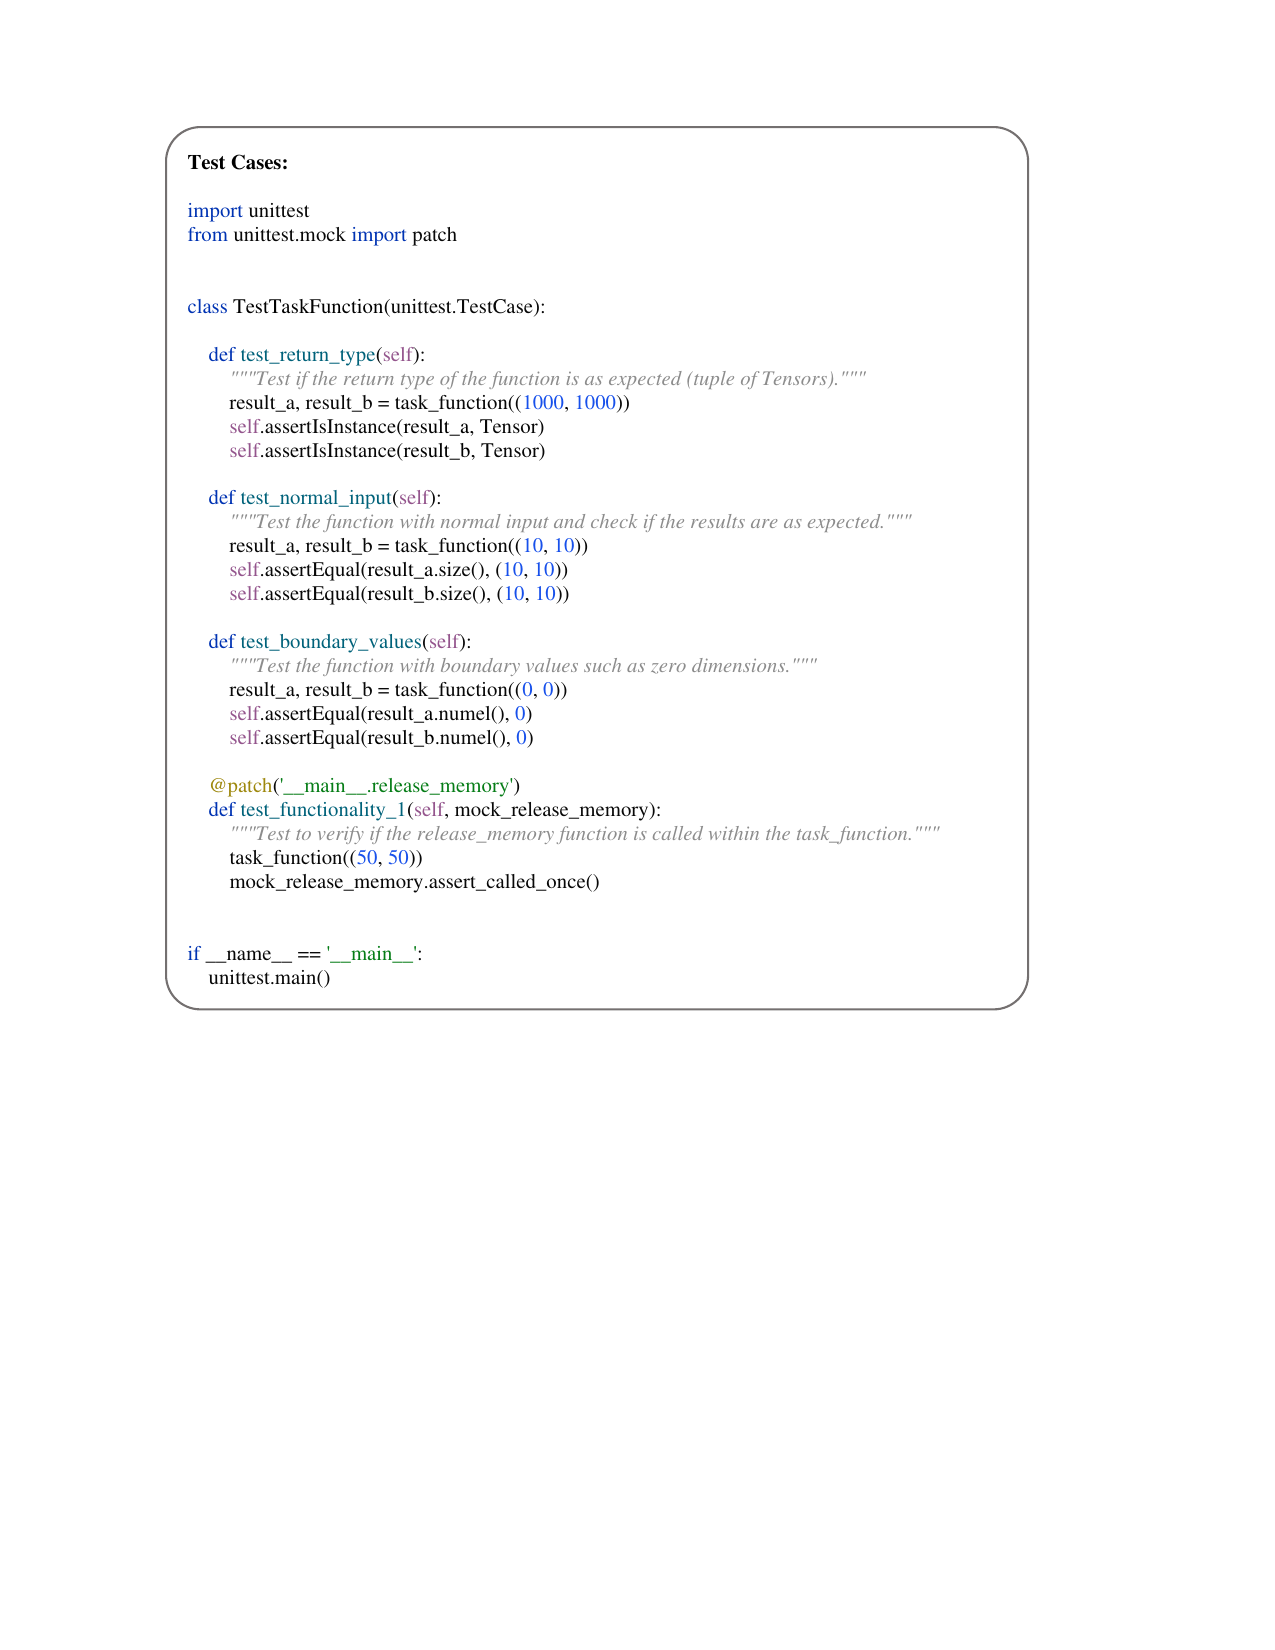}
    \caption{An example of test cases}
    \label{fig:test_cases}
\end{figure*}


\section{Example Analysis}
\label{apd:negative_example}
\subsection{Error Analysis of GPT4-o}
\label{subapd:ea}
Despite GPT4-o achieving superior performance in general evaluation, it still encounters errors in 30\% of instances. We provide several negative examples in Figure~\ref{fig:ne1}, Figure~\ref{fig:ne2}, Figure~\ref{fig:ne3}, and Figure~\ref{fig:ne4}.


\begin{figure}[t]
    \centering
    \includegraphics[width=1.0\textwidth, bb=0 0 741.47 273.6]{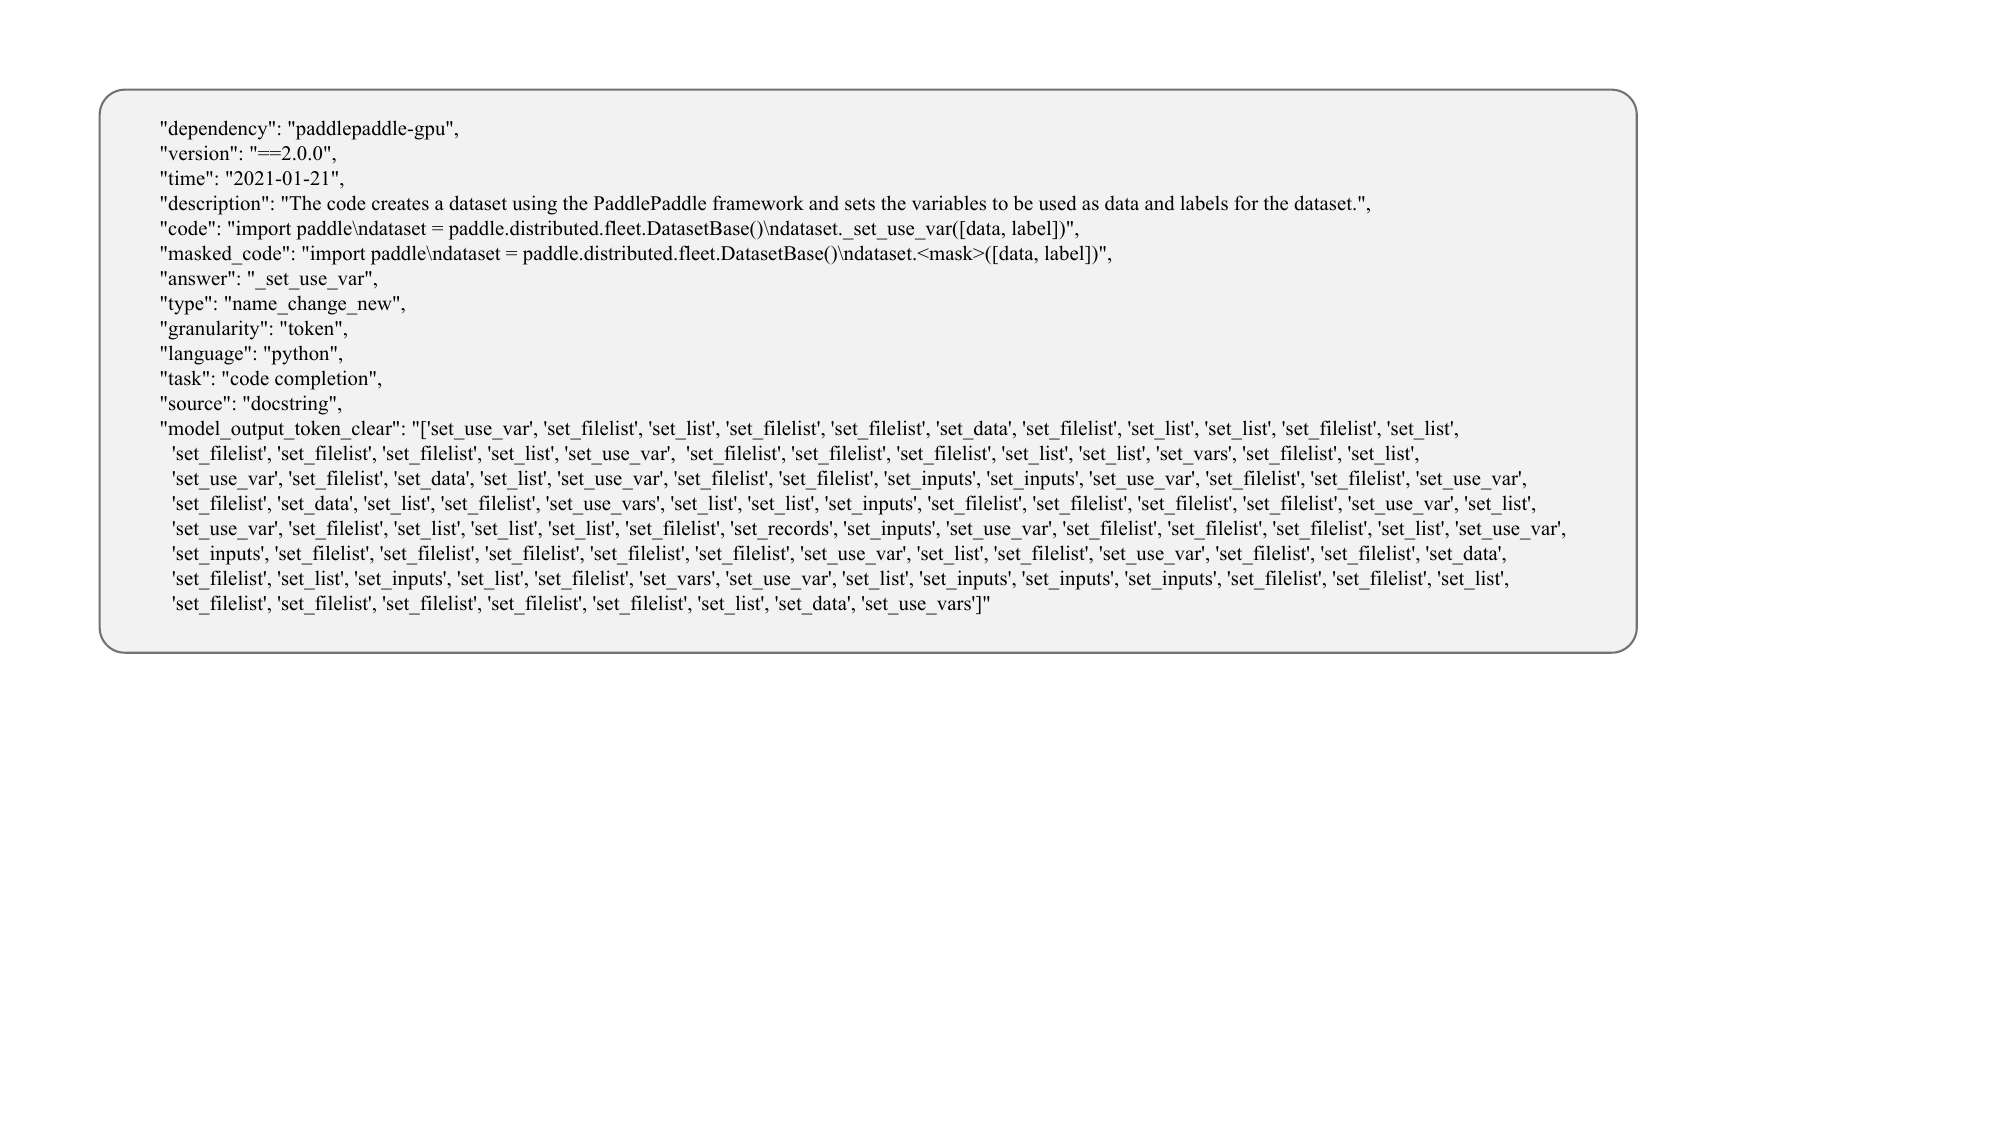}
    \caption{The first negative example of GPT-4o on token-level code completion.}
    \label{fig:ne1}
\end{figure}

\begin{figure}[t]
    \centering
    \includegraphics[width=1.0\textwidth, bb=0 0 741.47 225.6]{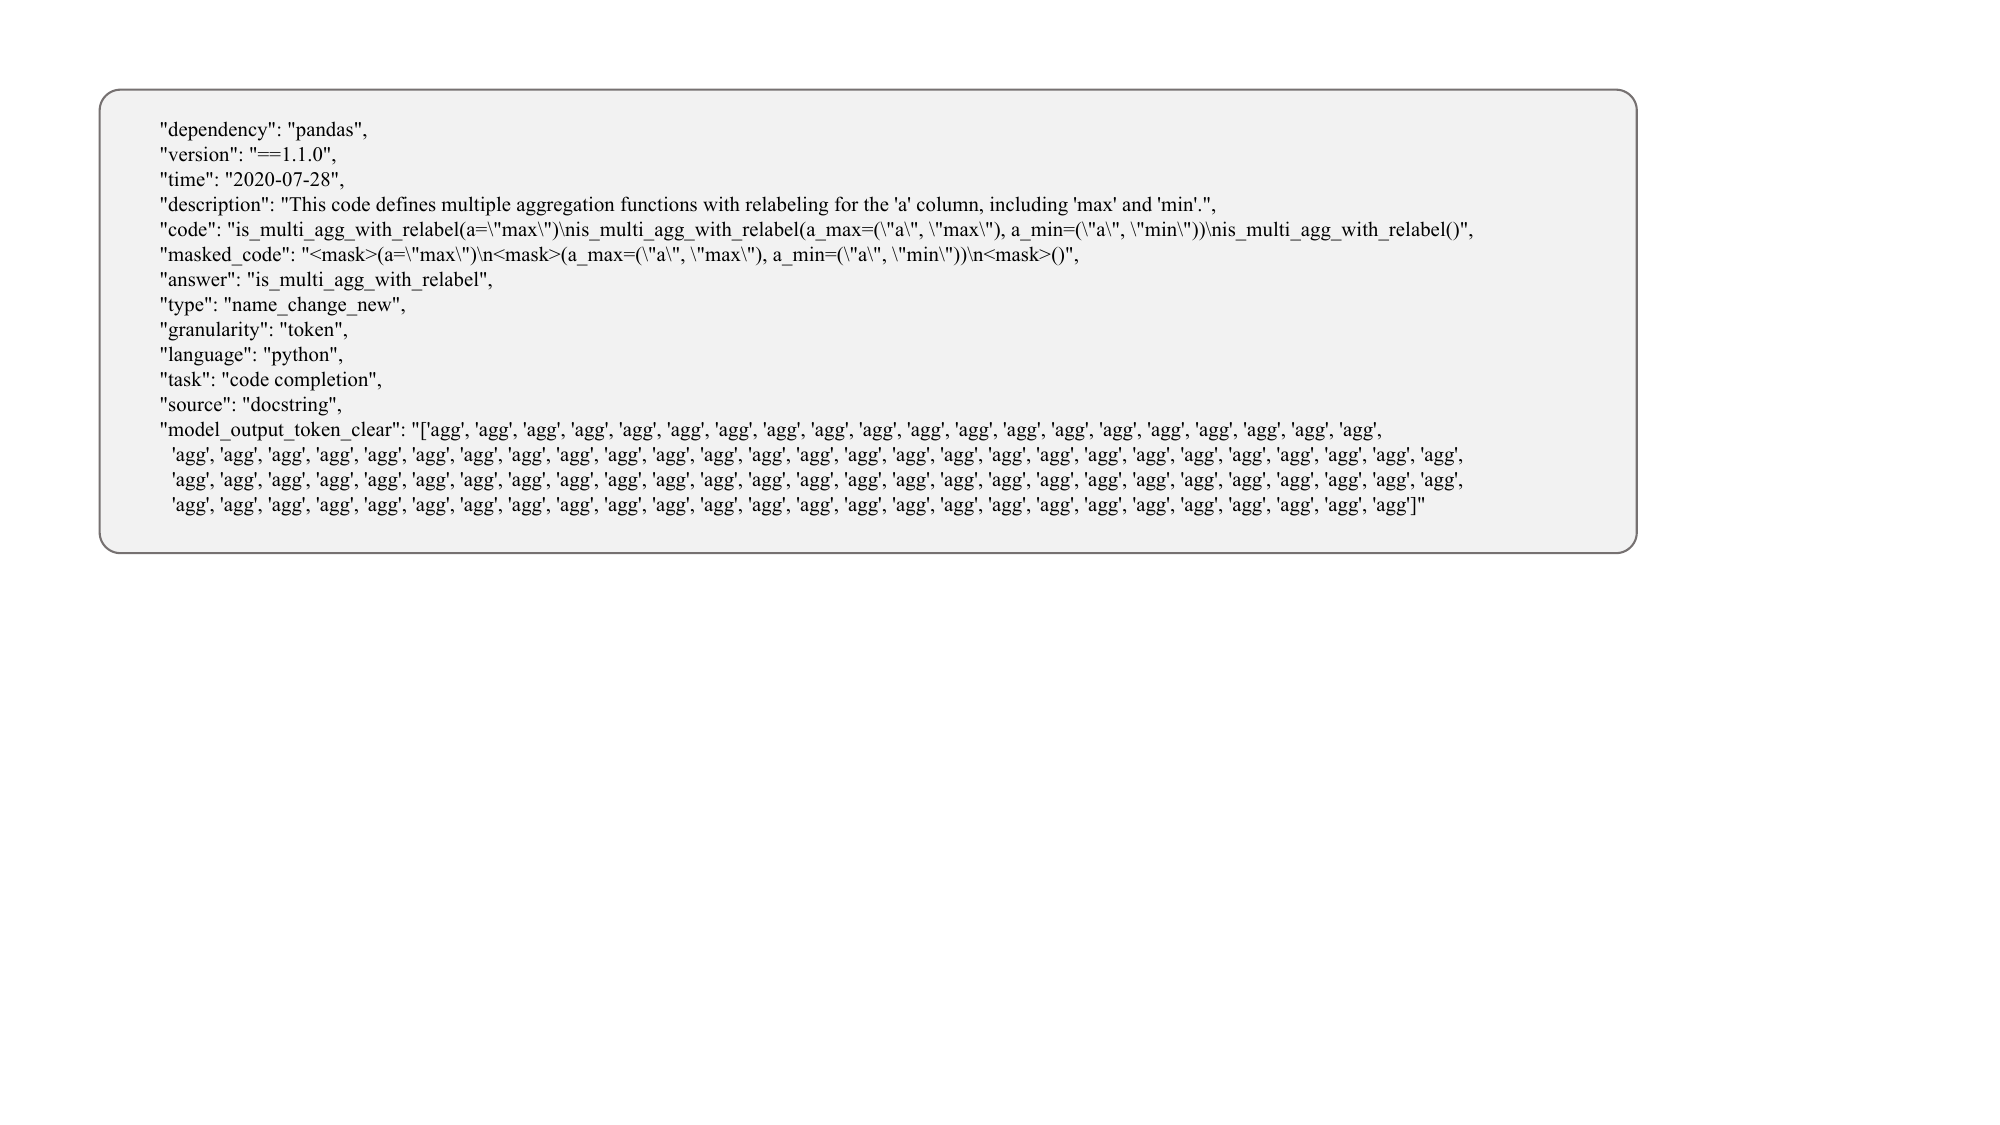}
    \caption{The second negative example of GPT-4o on token-level code completion.}
    \label{fig:ne2}
\end{figure}


\begin{figure}[t]
    \centering
    \includegraphics[width=1.0\textwidth, bb=0 0 743.877 296.4]{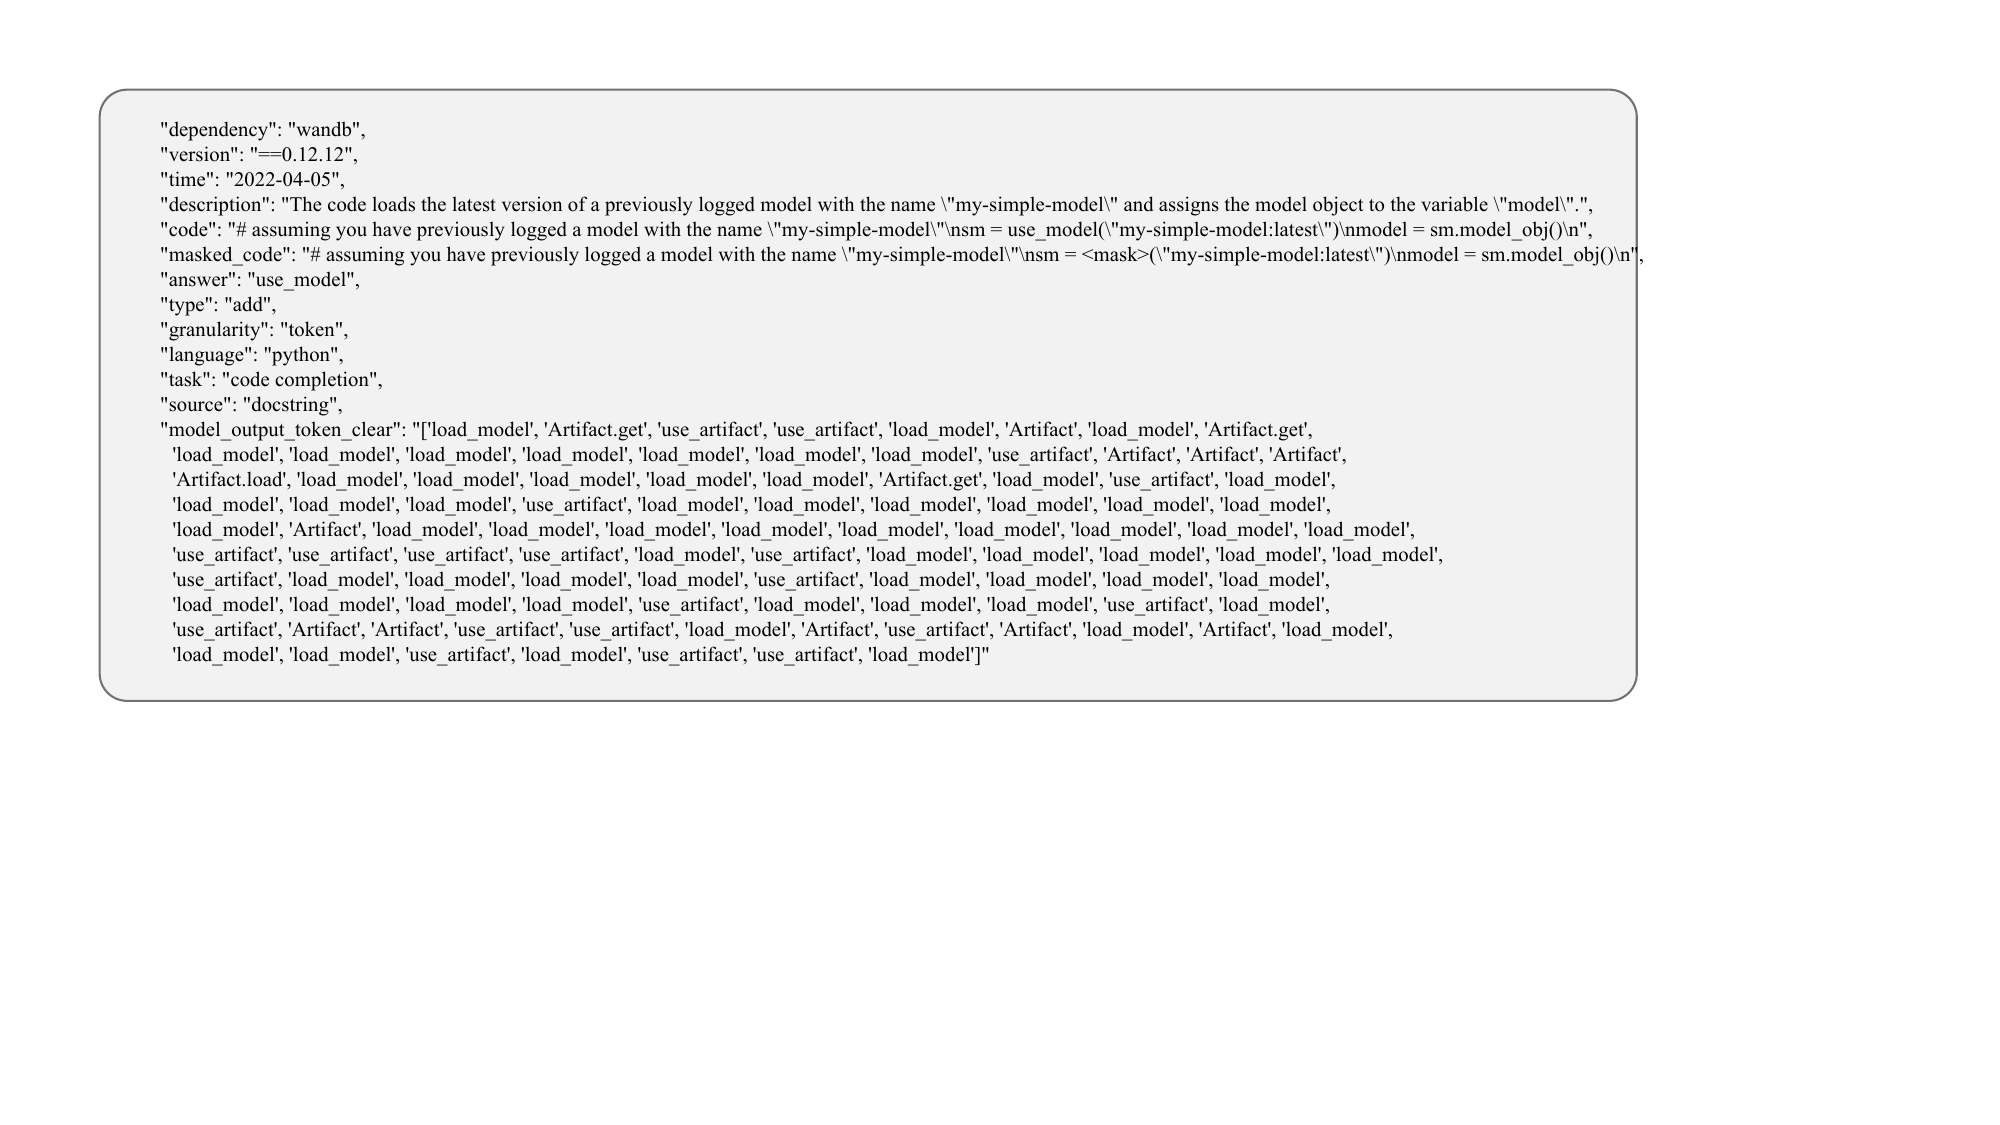}
    \caption{The third negative example of GPT-4o on token-level code completion.}
    \label{fig:ne3}
\end{figure}


\begin{figure}[t]
    \centering
    \includegraphics[width=1.0\textwidth, , bb=0 0 741.47 296.4]{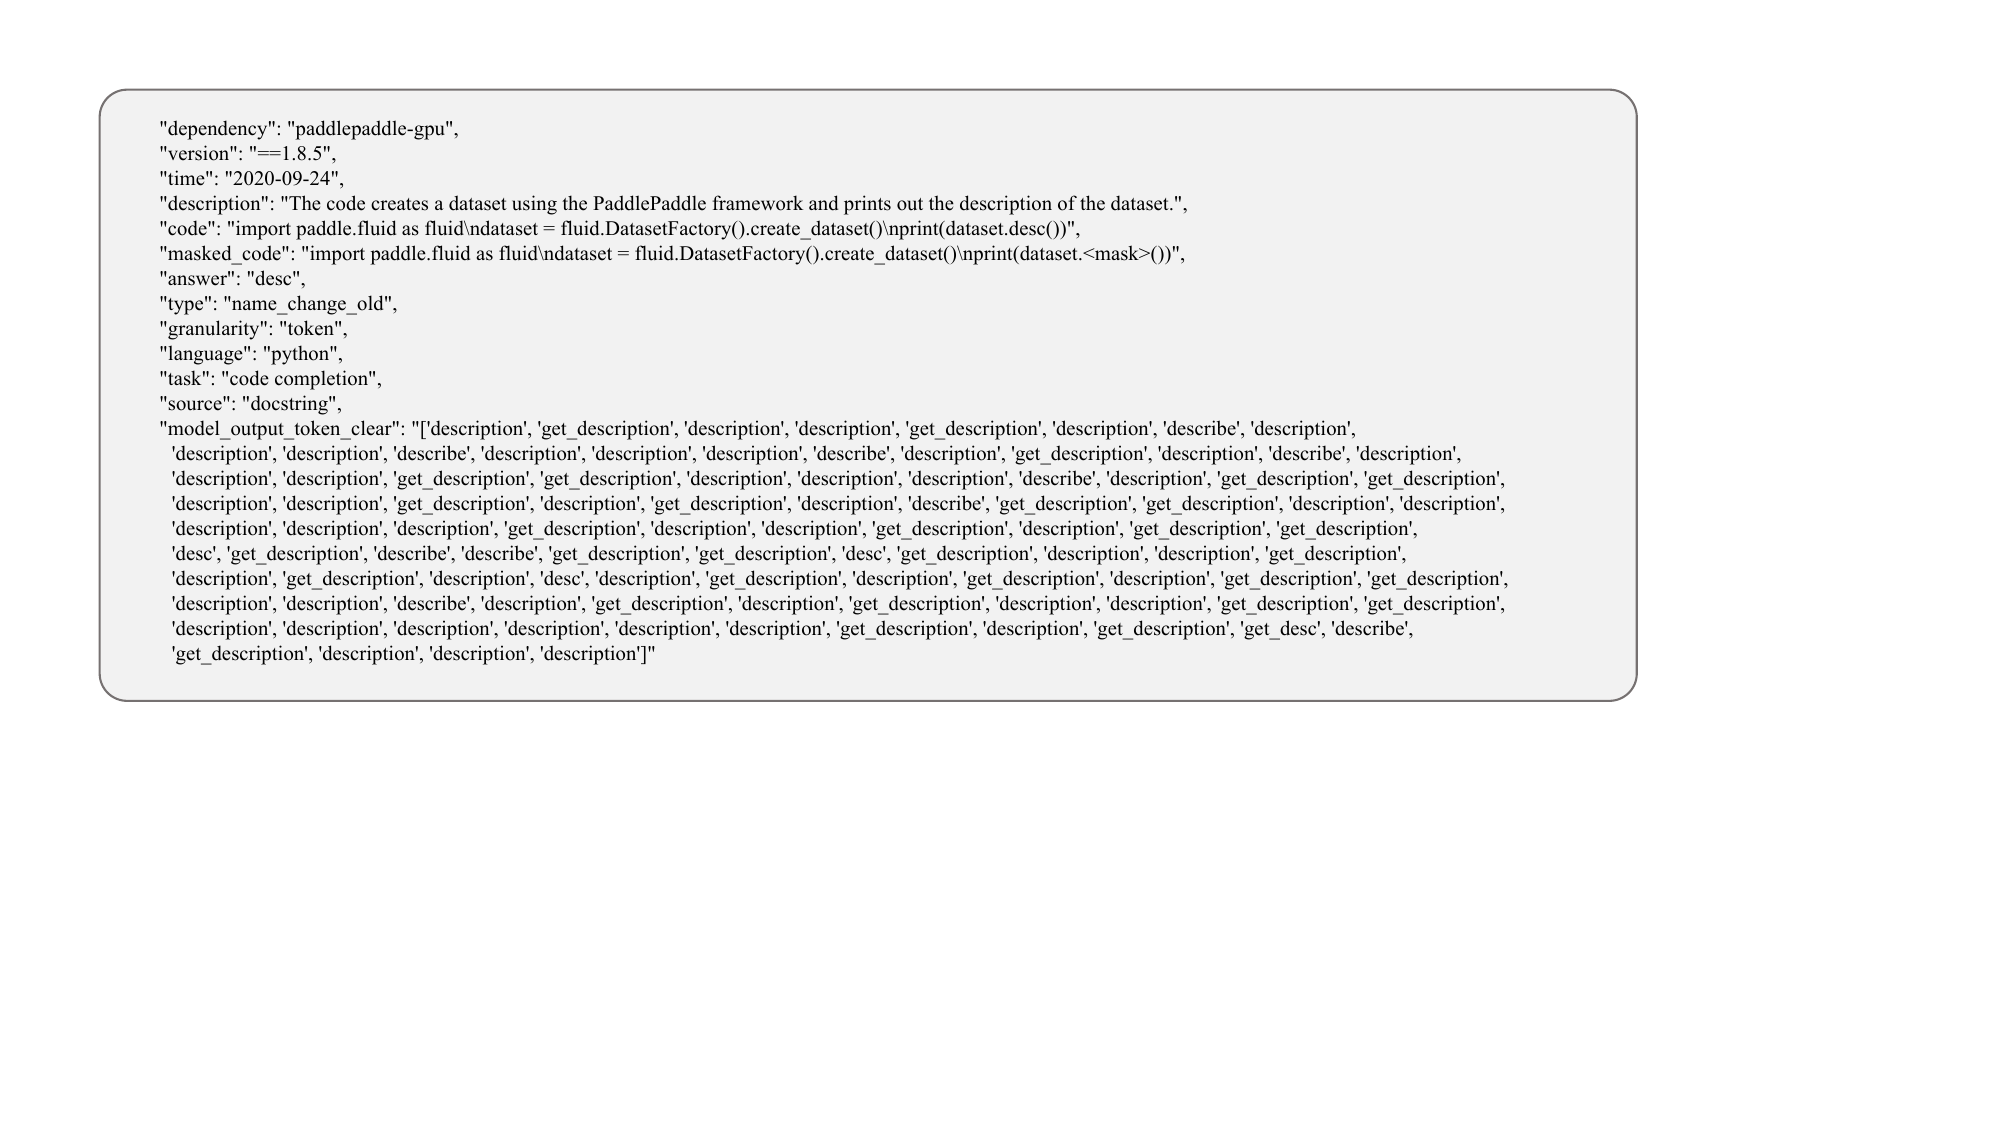}
    \caption{The fourth negative example of GPT-4o on token-level code completion.}
    \label{fig:ne4}
\end{figure}
